# Supplementary material for: Rayleigh-Plateau Instability on an angled and eccentric fiber: An alternative approach
Source: arXiv:2410.16949 source file (2026-04-29)
Supplement: Supplementary file 1 [file supplementary_material_v3.tex]

% ****** Start of file apssamp.tex ******
%
%   This file is part of the APS files in the REVTeX 4.2 distribution.
%   Version 4.2a of REVTeX, December 2014
%
%   Copyright (c) 2014 The American Physical Society.
%
%   See the REVTeX 4 README file for restrictions and more information.
%
% TeX'ing this file requires that you have AMS-LaTeX 2.0 installed
% as well as the rest of the prerequisites for REVTeX 4.2
%
% See the REVTeX 4 README file
% It also requires running BibTeX. The commands are as follows:
%
%  1)  latex apssamp.tex
%  2)  bibtex apssamp
%  3)  latex apssamp.tex
%  4)  latex apssamp.tex
%
\documentclass[reprint,
%superscriptaddress,
%groupedaddress,
%unsortedaddress,
%runinaddress,
%frontmatterverbose, 
%preprint,
%preprintnumbers,
%nofootinbib,
%nobibnotes,
%bibnotes,
 amsmath,amssymb,
 aps,onecolumn
%pra,
%prb,
%rmp,
%prstab,
%prstper,
%floatfix,
]{revtex4-2}

\usepackage{graphicx}% Include figure files
\usepackage{dcolumn}% Align table columns on decimal point
\usepackage{bm}% bold math
\usepackage{hyperref}% add hypertext capabilities
\usepackage[mathlines]{lineno}% Enable numbering of text and display math
%\linenumbers\relax % Commence numbering lines
%\usepackage[showframe,%Uncomment any one of the following lines to test 
%%scale=0.7, marginratio={1:1, 2:3}, ignoreall,% default settings
%%text={7in,10in},centering,
%%margin=1.5in,
%%total={6.5in,8.75in}, top=1.2in, left=0.9in, includefoot,
%%height=10in,a5paper,hmargin={3cm,0.8in},
%]{geometry}
\usepackage{xcolor}

\begin{document}

\preprint{APS/123-QED}

\title{Rayleigh-Plateau Instability on an angled and eccentric wire}% Force line breaks with \\
%\thanks{Droplets are much larger than capillary length}%
\author{Dilip Kumar Maity$^1$}\email{dilip.maity@kaust.edu.sa} 
\author{Christopher Wagstaff$^2$} \author{Sandip Dighe$^1$} \author{Tadd Truscott$^1$}\email{taddtruscott@gmail.com}

\affiliation{ $^1$Department of Mechanical Engineering, Physical Science and Engineering Division, King Abdullah University of Science and Technology, Thuwal, 23955, Kingdom of Saudi Arabia. \\
$^2$Department of Chemical Engineering, King Abdullah University of Science and Technology, Thuwal, 23955, Kingdom of Saudi Arabia
}

\date{\today}% It is always \today, today,
             %  but any date may be explicitly specified

%\keywords{Suggested keywords}%Use showkeys class option if keyword
                            %display desired
\begin{center}
\Large    Supplementary Materials
  \vspace{5pt}
%    \rule{3in}{0.5}
  \vspace{4pt}
\end{center}

\maketitle

\section{Experimental Setup}

\begin{figure}[ht!]
\centering
\includegraphics[width=0.32\textwidth]{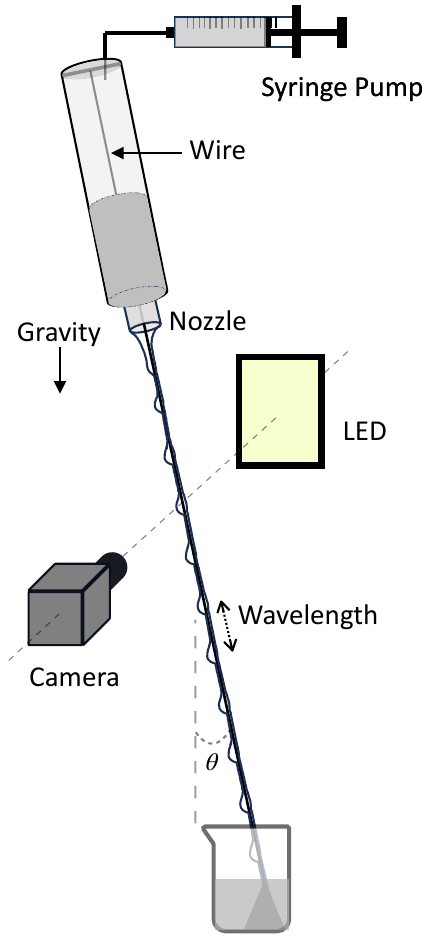}\label{supple_fig_1}
\caption{\label{fig_schematic} \textbf{Rayleigh-Plateau instability on an angled wire.} (a) Schematic representation depicting the jet and bead shape at a $10^\circ$ angle ($\theta$) from the vertical with the wire positioned at the center of the nozzle ($e_n=0$).}
\end{figure}

\section{Volume calculation}
% tasks 1. Draw a schematic for volume calculation
We calculate the volume of an asymmetric bead using camera data from one camera angle, which requires an elliptical assumption. Here we present the implication of that assumption. 

\begin{figure}[hb!]
\centering
\includegraphics[width=0.45\textwidth]{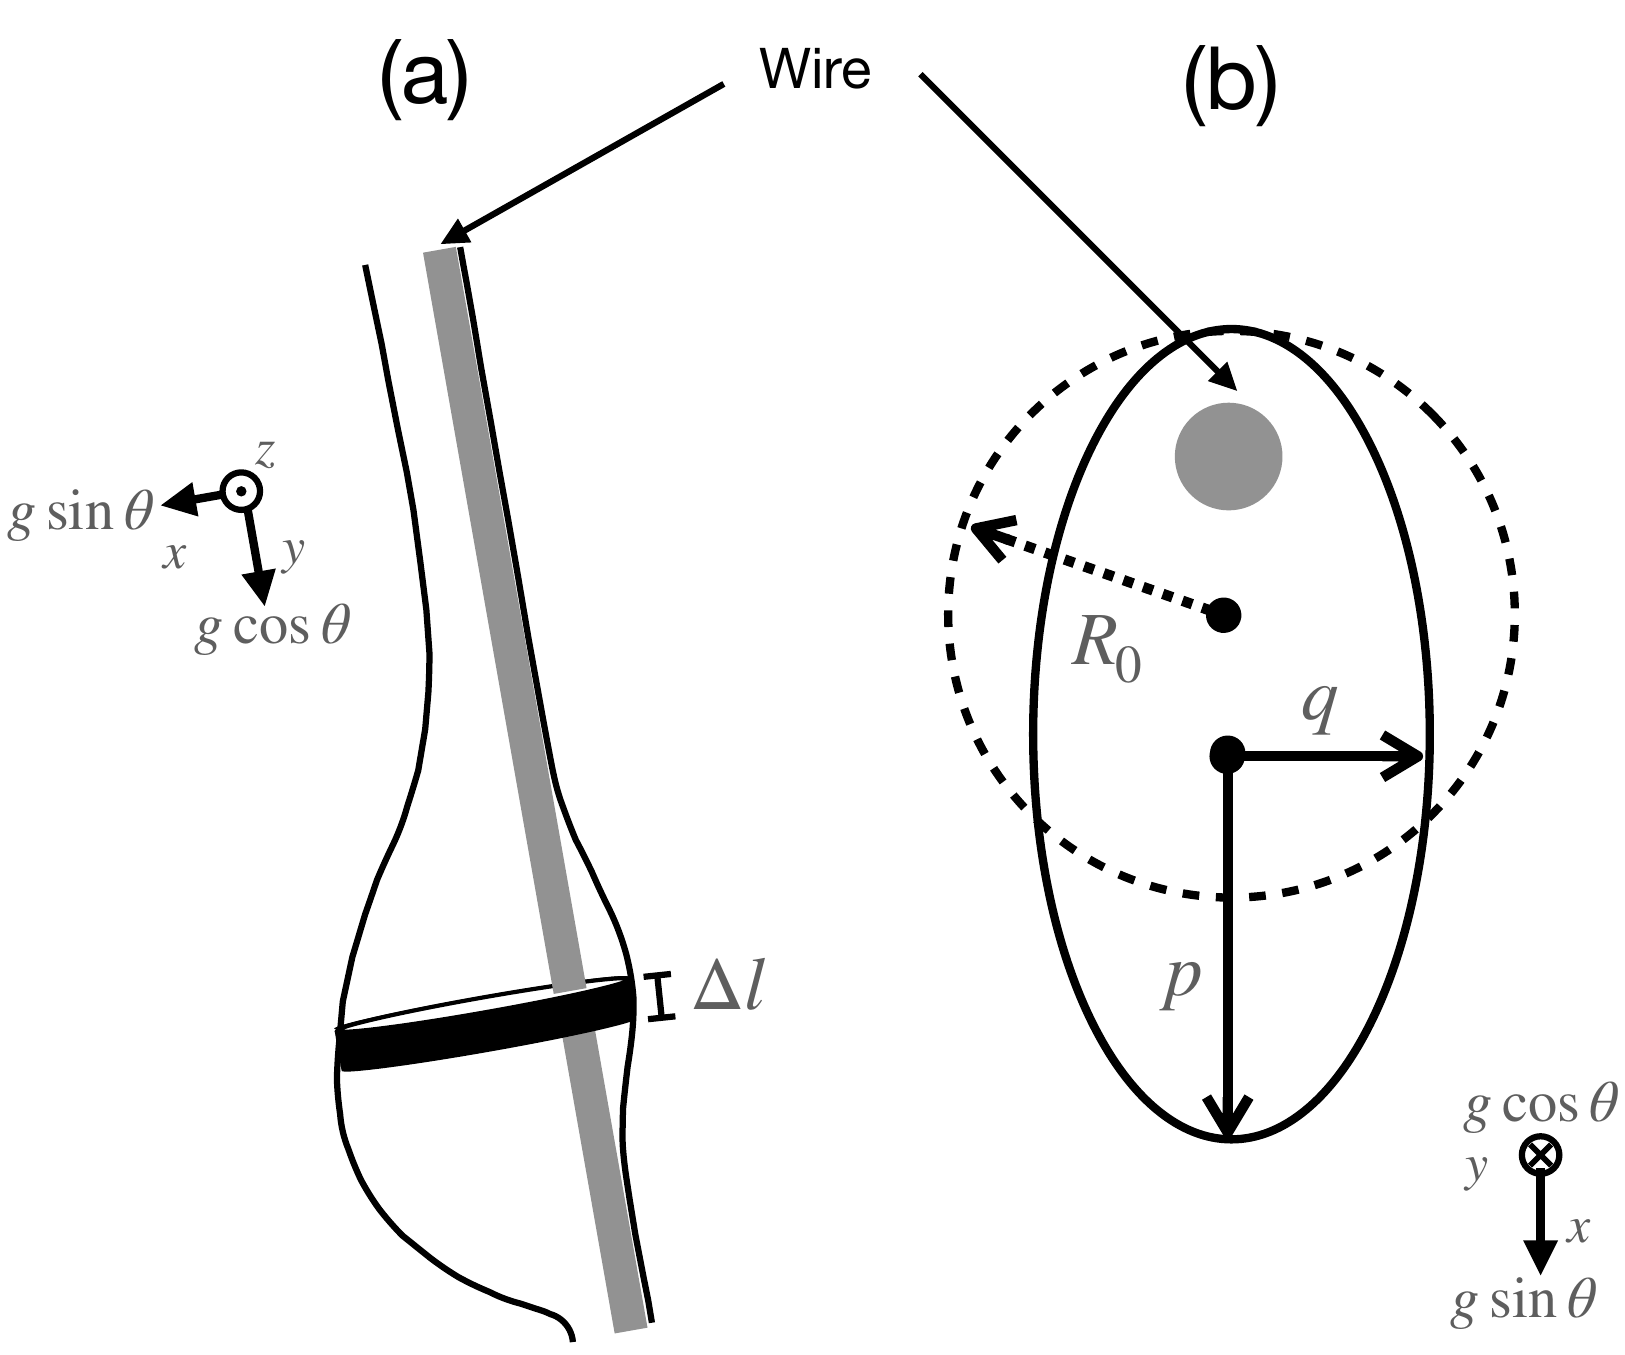}
\caption{\label{supple_fig_volume} \textbf{Volume calculation of liquid a bead.} schematic representation of (a) the side view a bead on an angled wire (b) the cross sectional view of a bead on an angled wire.}
\end{figure}

In the vertical configuration, the droplet exhibits axis-symmetric drops, resulting in a circular cross-sectional view. Conversely, for angled wires, the cross-sectional view takes an asymmetric  shape (assumed to be elliptical). Refer to supplementary Figure~S 2  for a visual representation of an angled bead. The bead volume is determined by treating the entire droplet as the sum of small ellipsoidal cross-sectional disks with thickness $\Delta l$ (Figure~S 2a). The cross-section of disk-shaped fluid elements undergo deformation from a circular shape to an ellipse shape as there is a component of gravity along the vertical direction of the wire when $\theta\neq 0$ (Figure~S 2b). Therefore, we assume the work performed by gravity on the bead volume along the $x$-direction of the wire is stored as excess surface energy (i.e., an ellipse) when compared to $g sin\theta \rightarrow 0$ and can be written as
\begin{equation}\label{ec}
\pi p q \Delta l \rho (p-R_0) g sin{\theta}=\pi (p+q)\Delta l\sigma-2\pi R_0 \Delta l \sigma,
\end{equation}
where $p$ and $q$ are the major and minor axis of the deformed elliptical disk, and $R_0$  is the undisturbed radius of the circular disk. Further, the conservation of the volume suggests 
\begin{equation}\label{vc}
R_0=\sqrt{p q}
\end{equation}
Combining equations (\ref{ec}) and (\ref{vc})
reveals
\begin{equation}\label{qe}
(\sqrt{p/q})^2-\sqrt{p/q}-\frac{\rho g p^2 sin{\theta}}{\sigma}=0.
\end{equation}
Therefore,
\begin{equation}\label{beq}
q=\frac{4p}{({{1+{\sqrt{1+\frac{4\rho g p^2 sin{\theta}}{\sigma}}}}})^2}
\end{equation}

We then determine $p$ through the analysis of the image obtained via the camera, and the value of $q$ is computed from Equation~\ref{beq}. Then we  compute the volume of the individual elliptical disk segments from 
\begin{equation}\label{icv}
\forall_i =\rho \pi p_i q_i \Delta l,
\end{equation}
where $\Delta l$ represents the length of a pixel. We then perform a numerical integration across the entire bead to obtain the overall volume of the bead as
\begin{equation}\label{ic}
\forall=\sum_i{\forall_i}=\sum_i{\rho \pi p_i q_i \Delta l}.
\end{equation}

\section{Results for different wire diameters and viscosity}

\begin{figure}[ht!]
\centering
\includegraphics[width=0.9\textwidth]{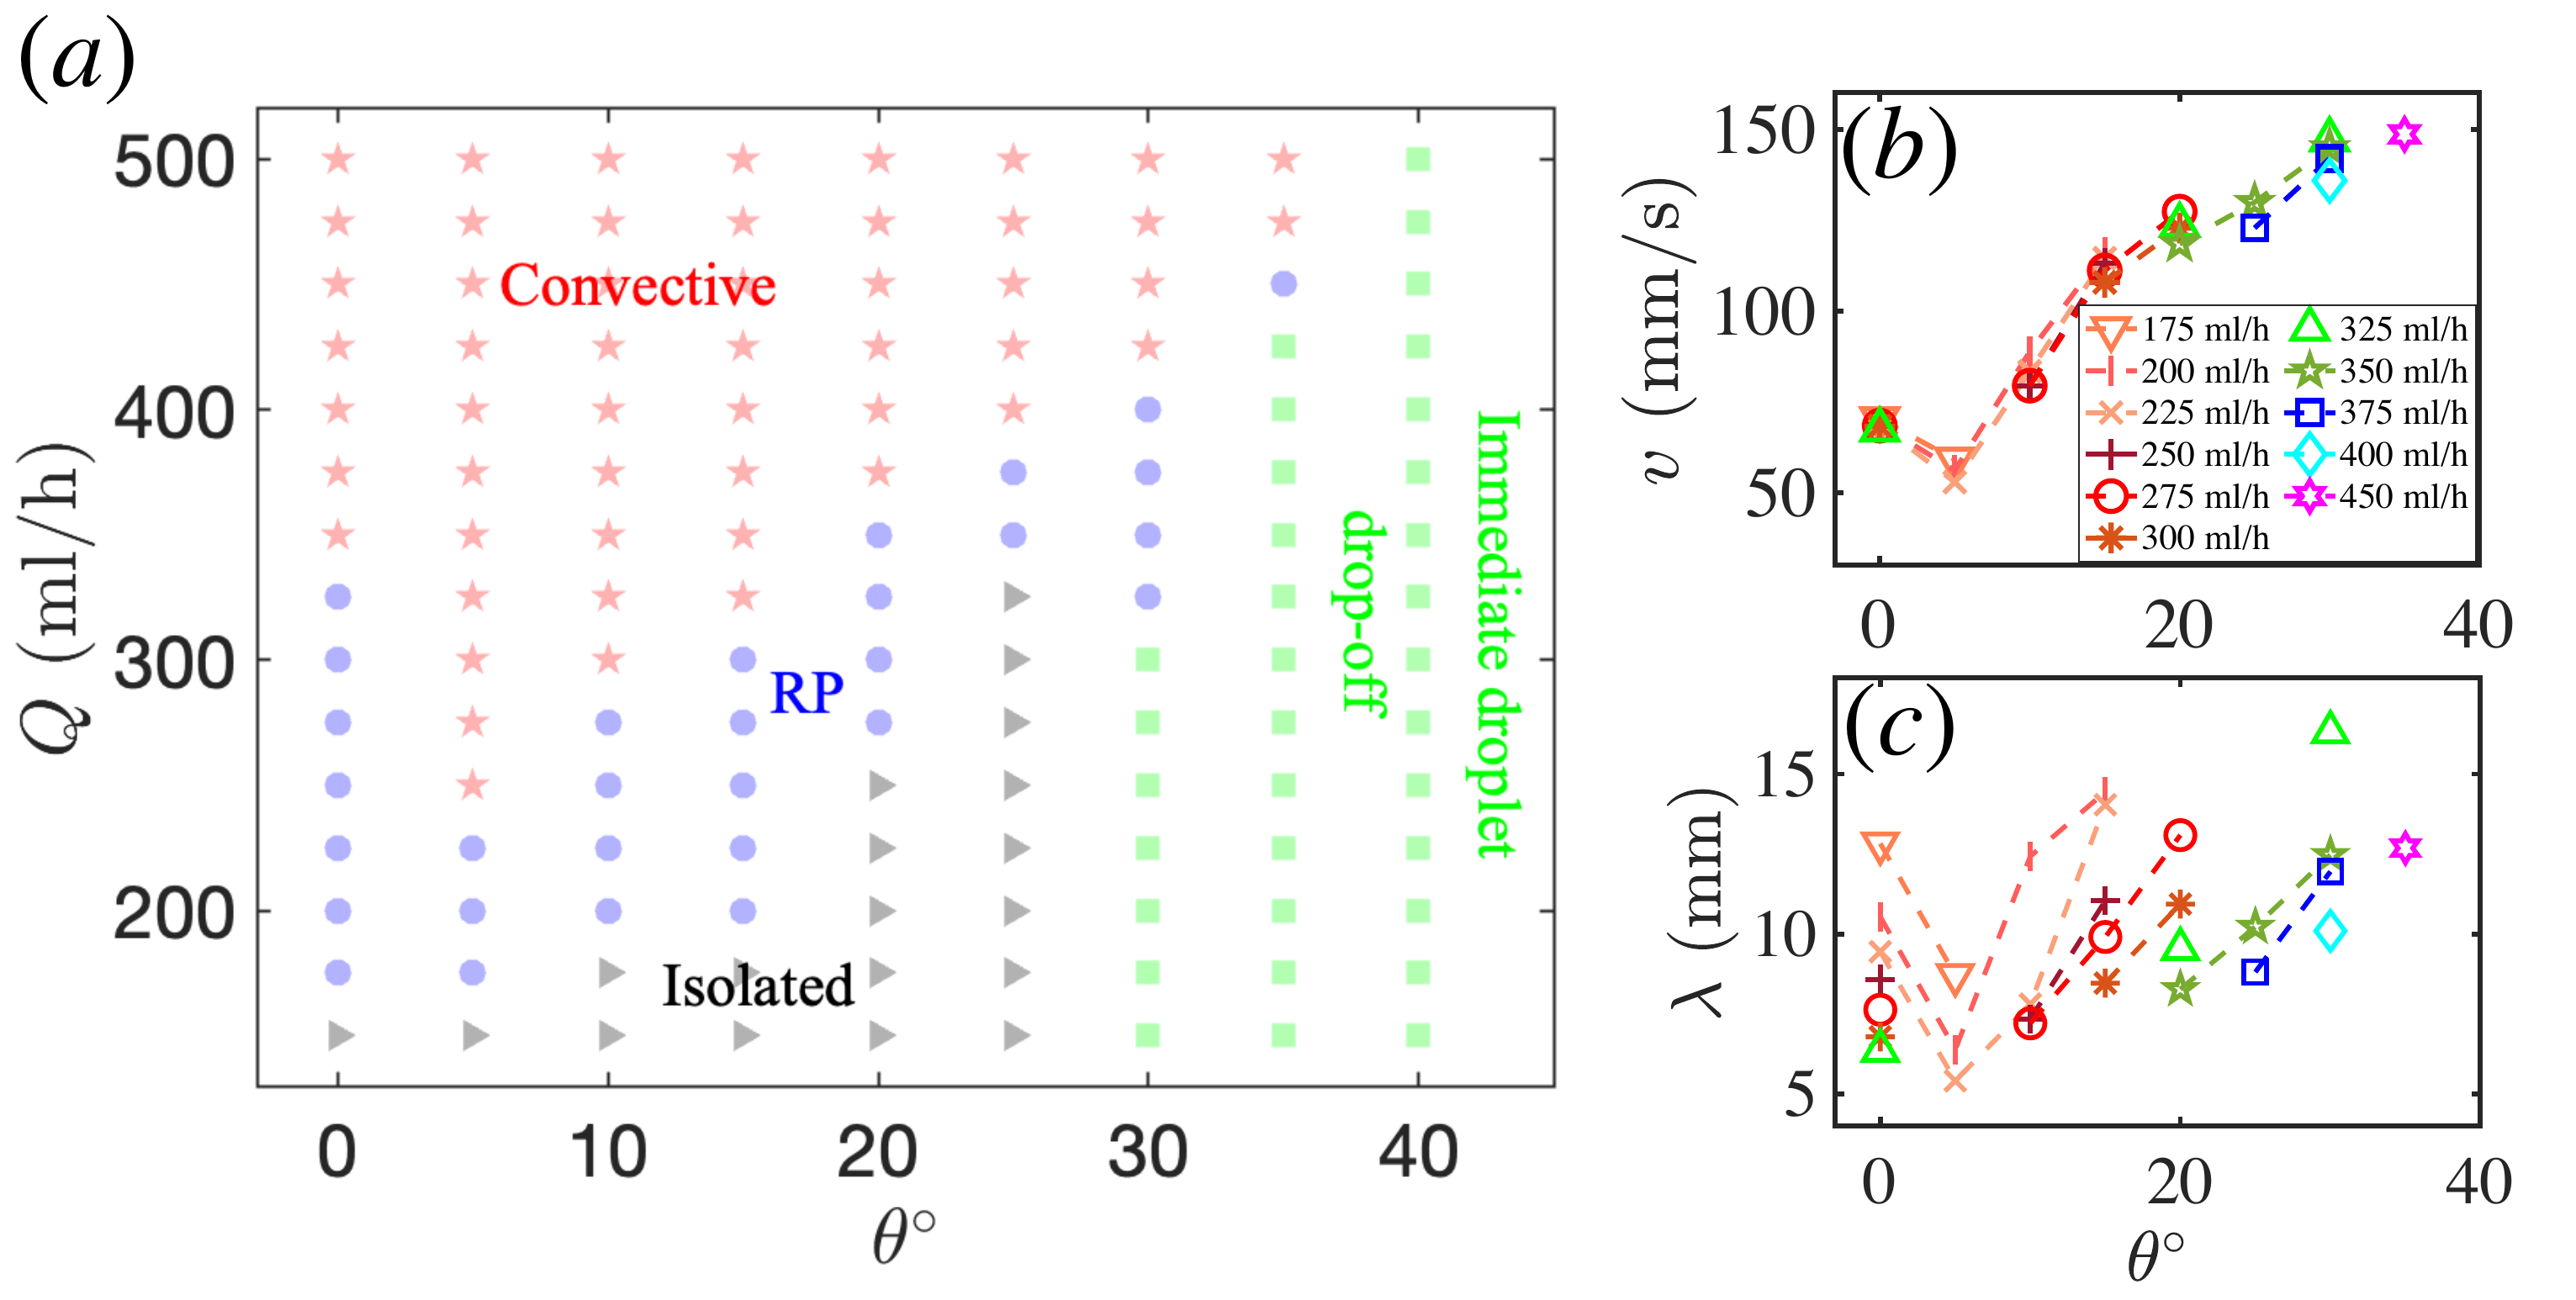}
\caption{\label{supple_fig3} For $r=0.15$ mm $\&$ viscosity = 50 cSt (a) Regime map (b) Velocity and (c) Wavelength variation in the Rayleigh-Plateau regime.}
\end{figure}

\begin{figure}[hb!]
\centering
\includegraphics[width=0.9\textwidth]{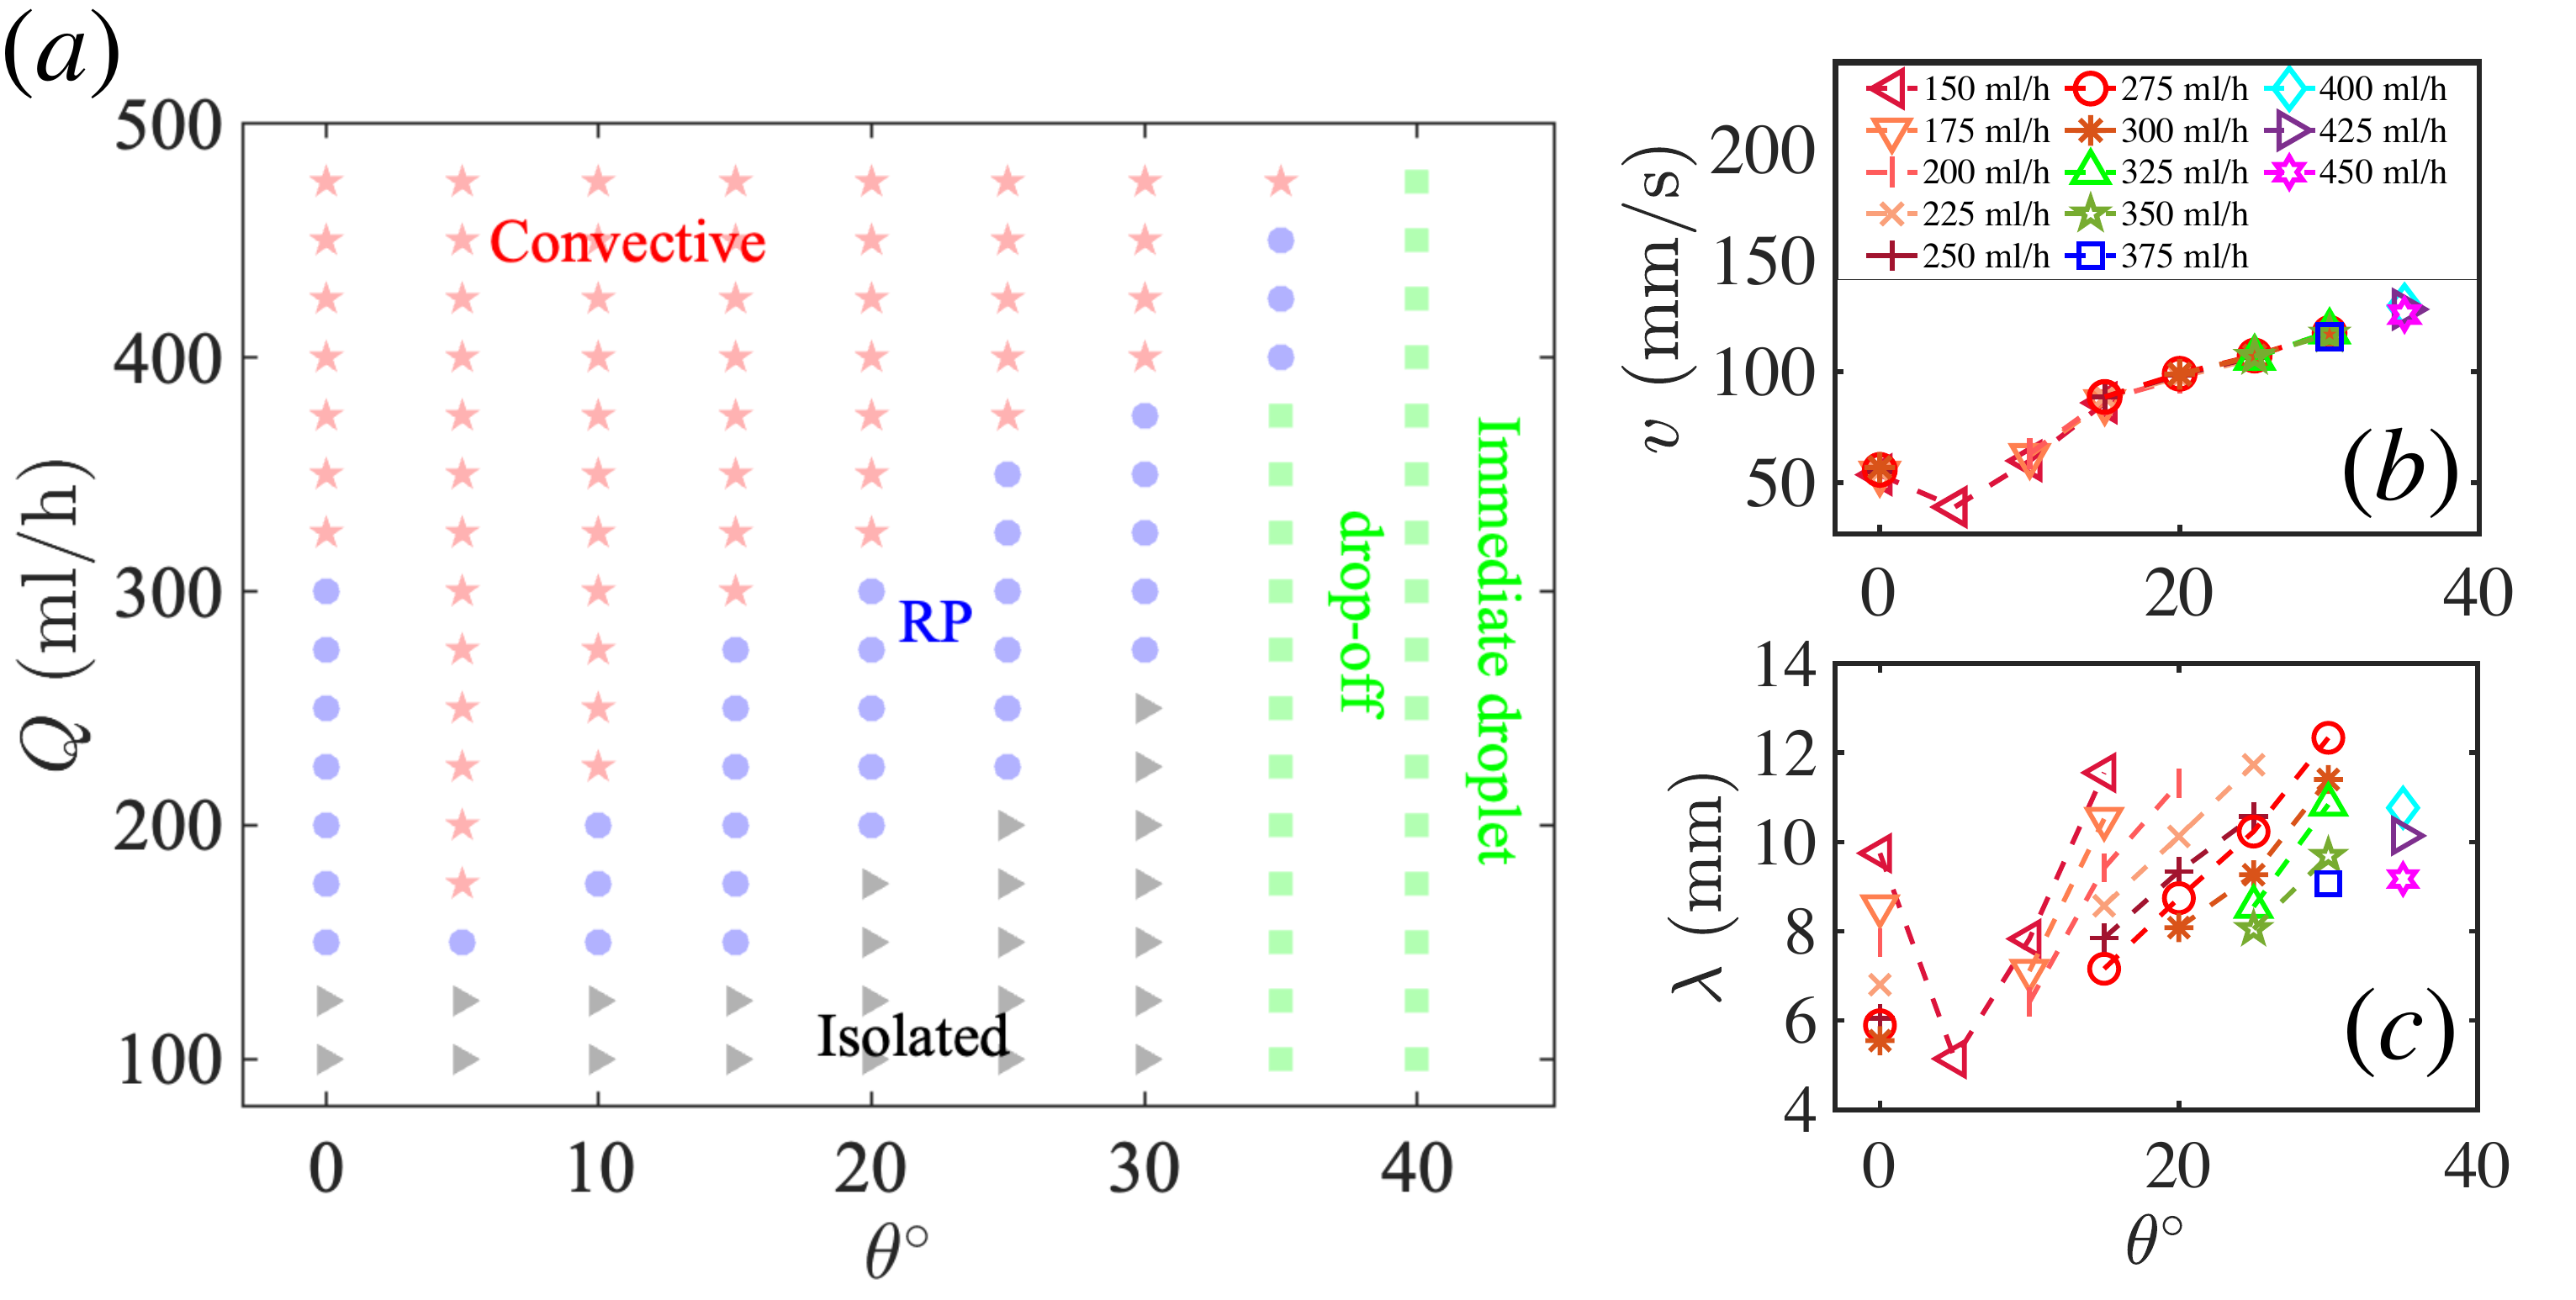}
\caption{\label{supple_fig4} For $r=0.2$ mm $\&$ viscosity = 50 cSt (a) Regime map (b) Velocity and (c) Wavelength variation in the Rayleigh-Plateau regime.}
\end{figure}

\begin{figure}[ht!]
\centering
\includegraphics[width=0.9\textwidth]{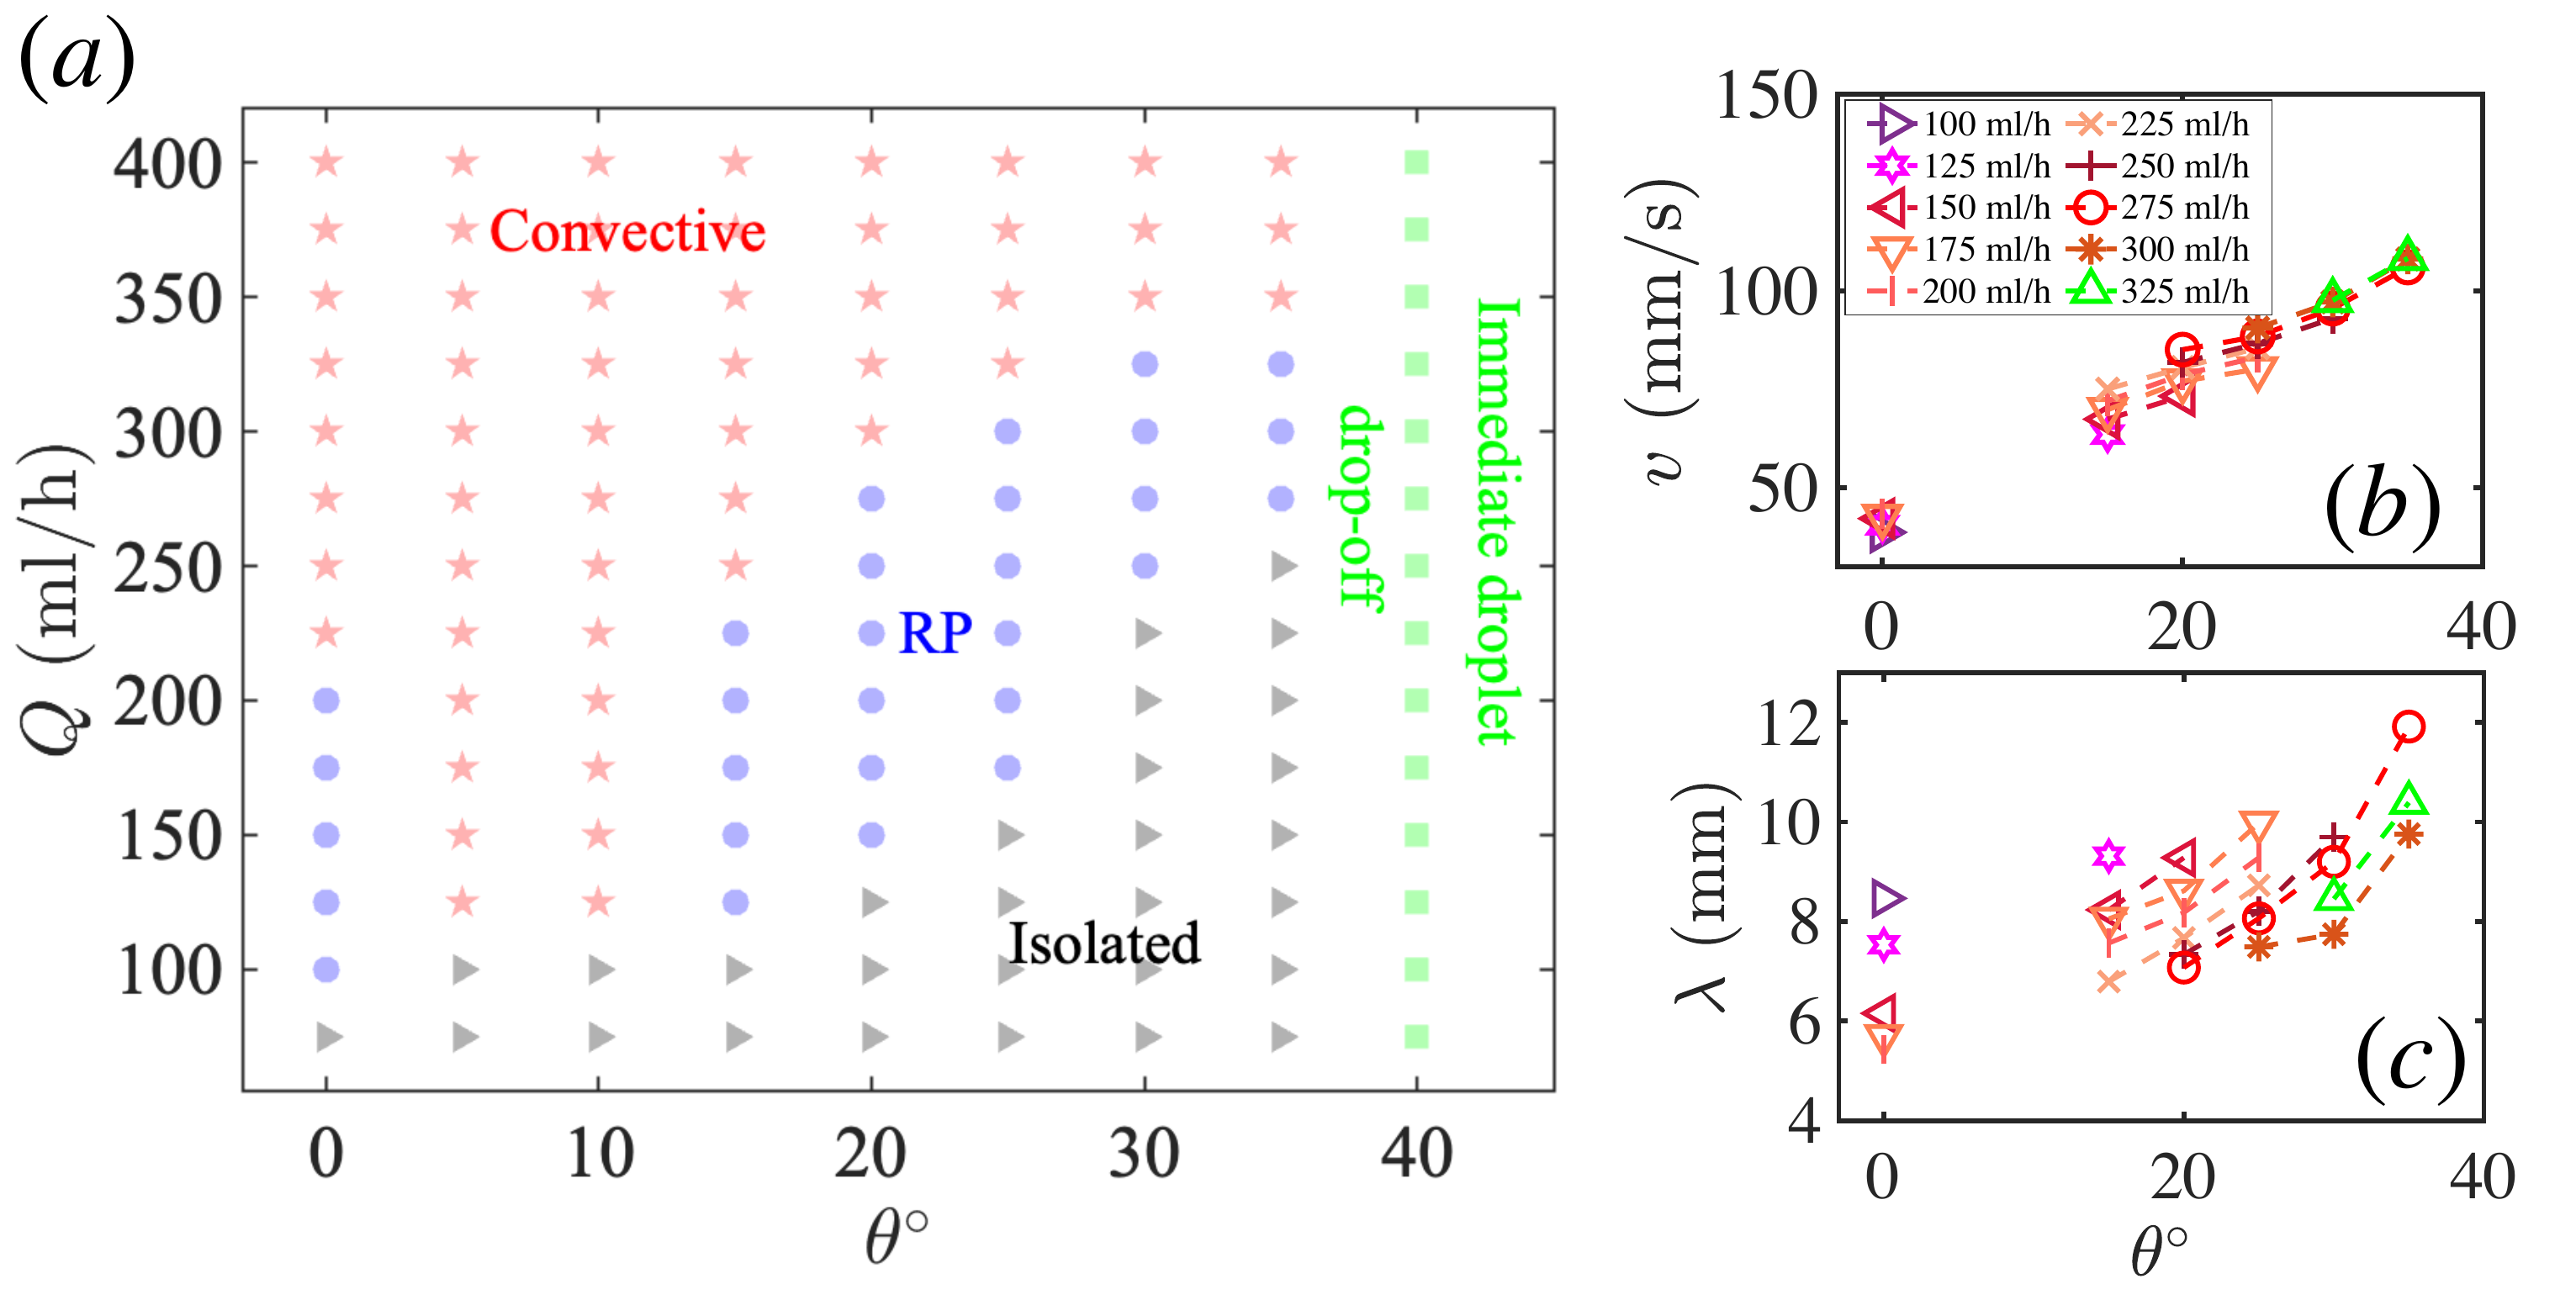}
\caption{\label{supple_fig5} For $r=0.25$ mm $\&$ viscosity = 50 cSt (a) Regime map (b) Velocity and (c) Wavelength variation in the Rayleigh-Plateau regime.}
\end{figure}

\begin{figure}[h!]
\centering
\includegraphics[width=0.9\textwidth]{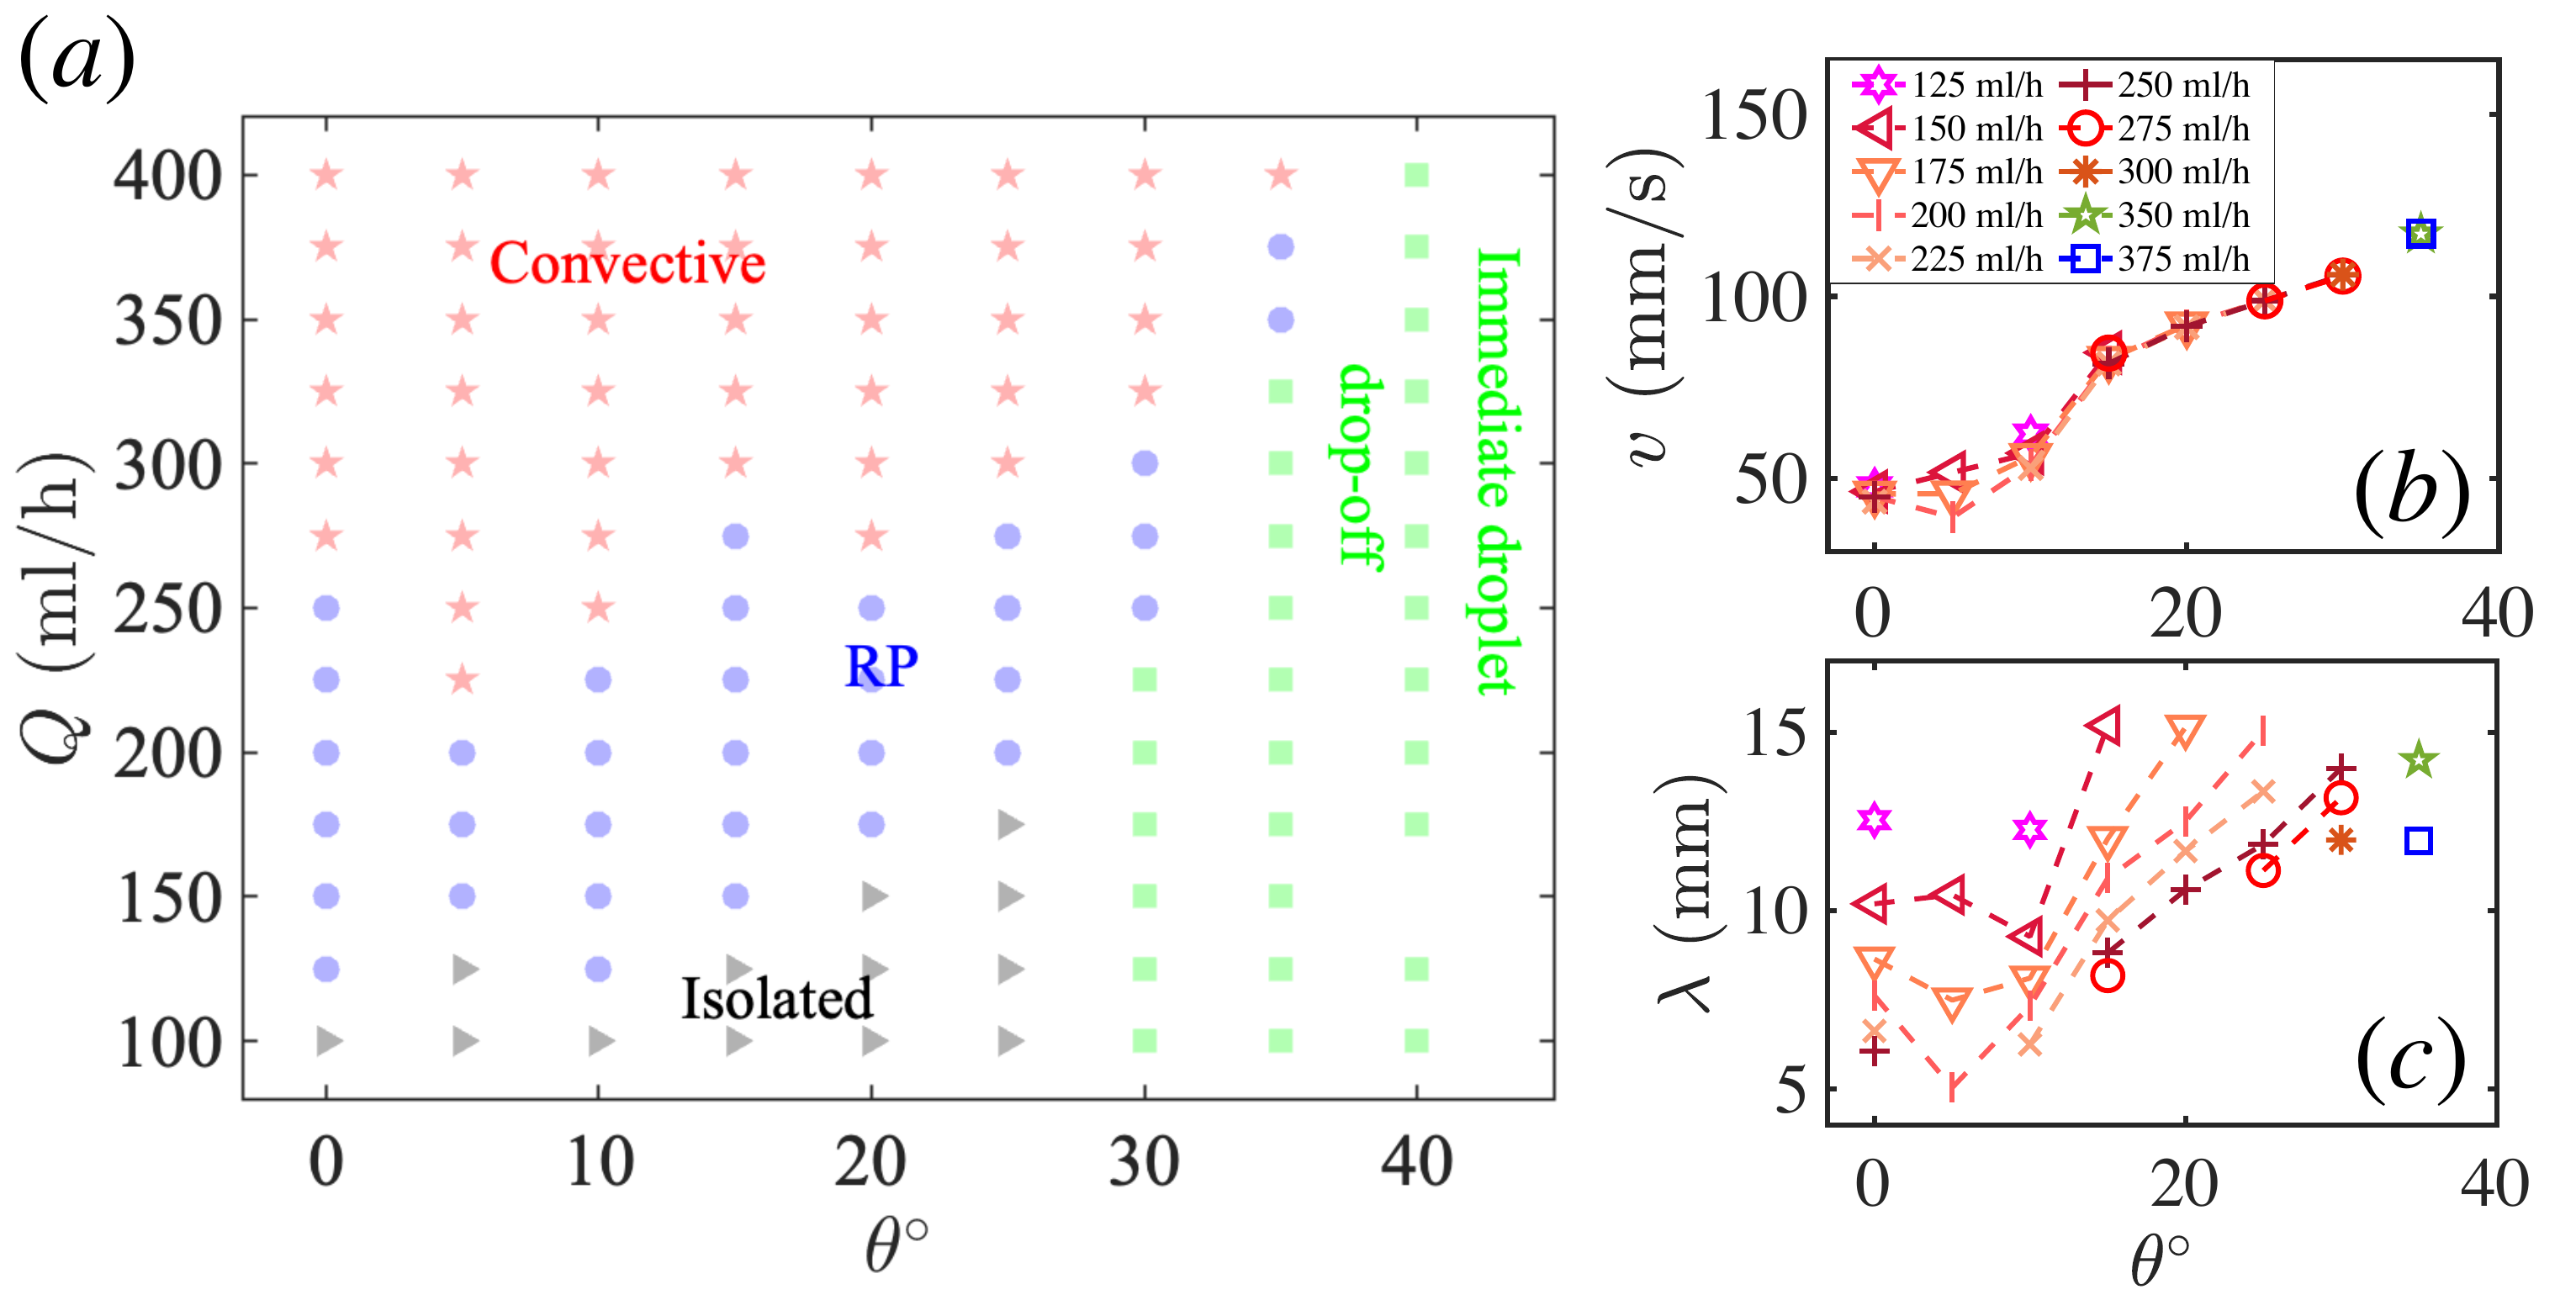}
\caption{\label{supple_fig6} For $r=0.1$ mm $\&$ viscosity = 100 cSt (a) Regime map (b) Velocity and  (c) Wavelength variation in the Rayleigh-Plateau regime.}
\end{figure}

\newpage
\section{Comparison of curvature-induced force}
\begin{figure}[h]
\centering
\includegraphics[width=0.45\textwidth]{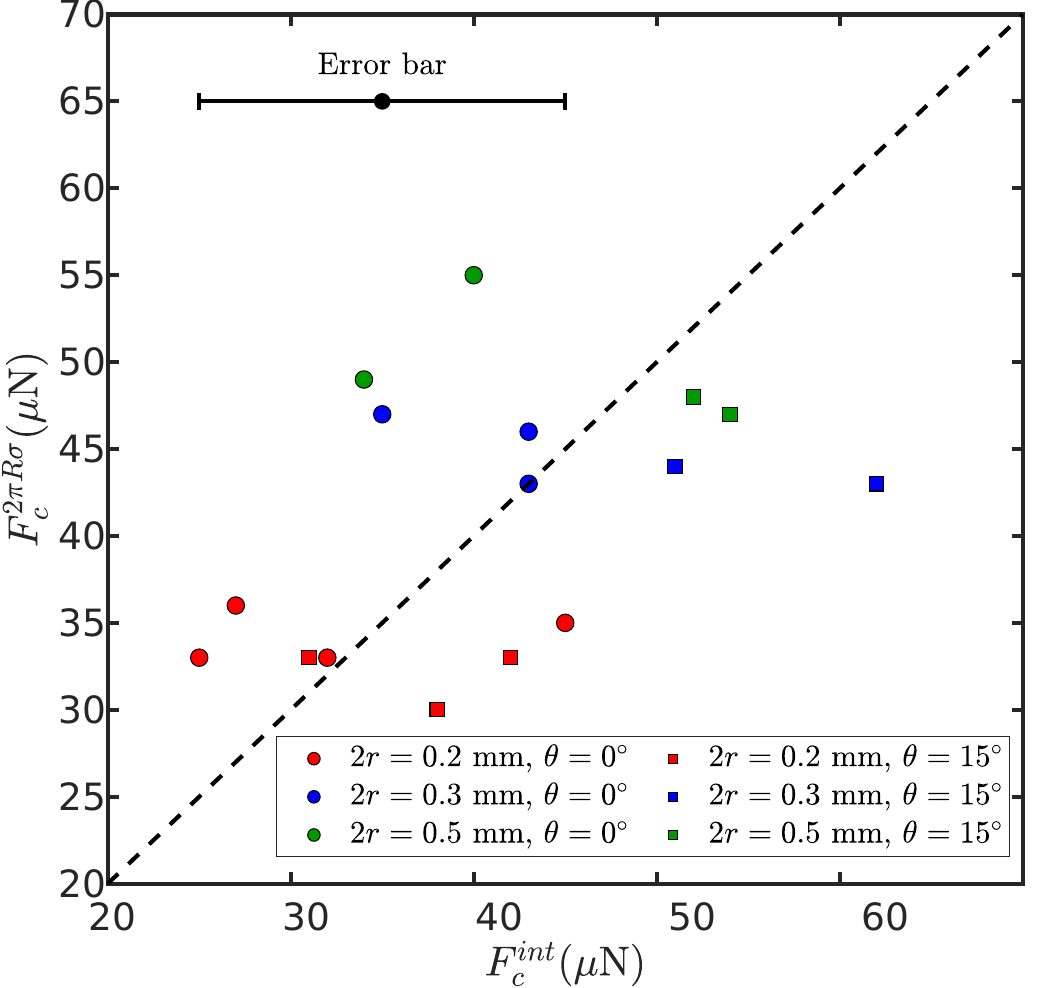}
\caption{\label{supple_fig7}Comparison of curvature induced force from integration $F_{c}^{int}$ and using $F_{c}^{2\pi R \sigma}=2\pi R \sigma$.}
\end{figure}

% \newpage
% \section{Without unknown for $F_c$}
\begin{figure}[!]
\centering
\includegraphics[width=0.45\textwidth]{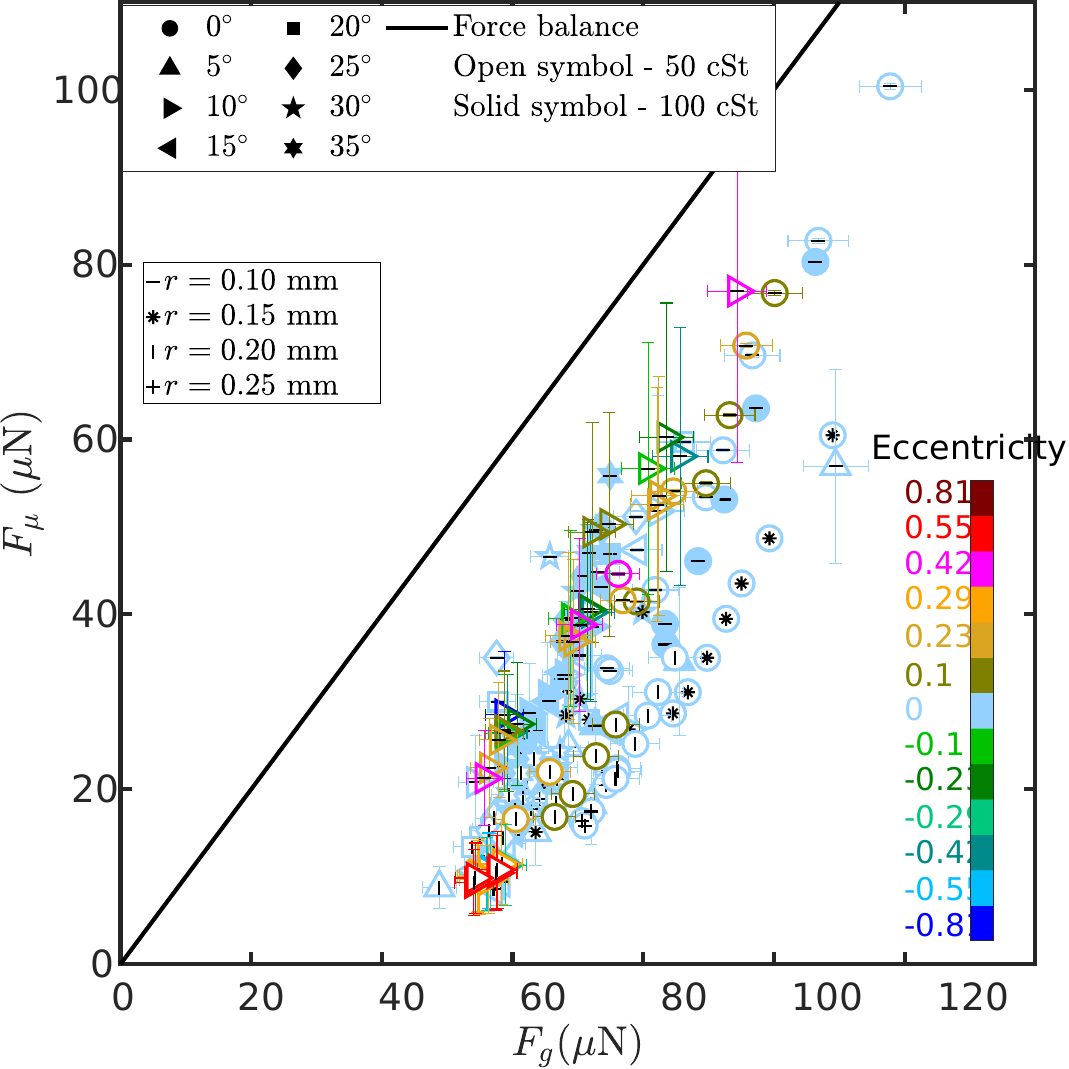}
\caption{\label{supple_fig8}The variation of the viscous force $F_{\mu}$ as a function of the gravitational force $F_{g}$ is presented for all cases, illustrating a offset from the expected force balance.
}
\end{figure}

\newpage
\section{Force due to curvature}
{
% As the droplets form a periodic and continuously connected train, the surface tension forces ($F_{\sigma}$) acting at the top and bottom boundaries of the control volume effectively cancel out, resulting in no net force.
When plotting $F_{g}$ versus $F_{\mu}$, we find only a partial agreement, with the data showing an offset from a clear balance between the forces of gravity and viscous dissipation given by Eq. 1 as shown in Fig.~S8 indicating that some additional contribution may be missing from the force balance. We wondered if perhaps the additional force could come from the asymmetry of the curved surface of the droplets in the experiment shown in Fig.~S9~a\&b. If we assume that the Laplace pressure is perhaps the source of the missing force we can write something similar to \cite{blackmore1985surface} \begin{equation}
F_{c}= \int_{A}\Delta F_c=\int_{A}p \hat n \cdot \hat z dA = \sigma\int_{A}\hat n \times \hat{dA}
\label{eq:Fc_general}
\end{equation}
who showed that the integral of a this approximation is zero if the surface curvature integral is closed and the surface is in equilibrium. If we move forward anyway and assume that the wire ensures that the contour is not closed %If we move forward assuming that the wire ensures that the contour is not closed, then we can show that there is a net force in the upward direction if we directly integrate the RHS of Eq. 7 using images from Fig.S9~a\&b (as shown to the right of each image in Fig.S9~a\&b ) ), the result for each sample case is shown to the right of the images as a function of $\Delta z$. If we check this result for the data in this study we find that the integration can be well approximated by $2\pi R\sigma$ as shown in Fig.S7. }
%To improve the collapse across experimental conditions, we tentatively introduce an upward force term of the form \(F_{c} = 2\pi R \sigma\). 
%\cite{blackmore1985surface} abc.
%In our experiments, all of the droplets adopt an asymmetric shape, as shown in Fig.~S 9a,b, indicating a broken horizontal symmetry and the emergence of a net curvature force ($F_c$). 
%We observe internal circulation within the droplet in our case (see supplementary video 12 \cite{supple_video_2024}), resembling the behavior of a rolling droplet on an inclined surface \cite{backholm2020water, keiser2020universality,daniel2017oleoplaning}. This circulation arises due to viscous dissipation induced by the droplet’s curvature. The resulting force drives the circulation and contributes to the asymmetry in the droplet shape. Therefore, we assume that the curvature-induced force manifests as viscous dissipation.
%By balancing forces (Equation~\ref{eq_fb_1}) within the control volume, this curvature-induced upward force is estimated to be approximately $F_{c}=2\pi R \sigma$.
then the integration of the Laplace pressure ($p$) over the control volume yields the force
\begin{equation}
F_{c}= \int_{z=0}^{\lambda}\sigma \left( \frac{1}{R_1(z)} + \frac{1}{R_2(z)} \right) 2\pi R_1(z)  \sin{\phi(z)} dz
%\int_{A}\Delta F_c=\int_{A}p \hat n \cdot \hat z dA = \int_{z=0}^{\lambda}\sigma \left( \frac{1}{R_1(z)} + \frac{1}{R_2(z)} \right) 2\pi R_1(z)  \sin{\phi(z)} dz
%F_c= \int_{z=0}^{\lambda}\Delta F_c= \int_{z=0}^{\lambda}\sigma \left( \frac{1}{R_1(z)} + \frac{1}{R_2(z)} \right) 2\pi R_1(z)  \sin{\phi(z)} dz
\label{eq:Fc_general}
\end{equation}
where $R_1$ and $R_2$ are the principal radii of curvature at  $z$, $\hat n$ is the unit normal vector to the surface, and  $\phi$ is the angle between the surface normal and the horizontal. $\Delta F_{c}$ corresponds to the infinitesimal force acting over a length element $dz$.
 In Fig.~S 9a,b an image from the experiment is shown and we outline the radius of curvature ($R_2$) at one location and notice that the radii are larger at the top of the droplet than at the bottom. We also outline $R_1$ for both cases.  Next to the image we plot $\Delta  F_c$ vs. $z$ (direct correspondence to the image) to illustrate the variation of $F_c$ due to the asymmetry of the droplet. The data confirms that a force arises from the curvature of the droplet with a larger significance near the bottom of the droplet. We numerically integrate within the control volume to estimate the contribution of the curvature to the forces and find that the values are close to $2\pi R \sigma$ (see supplementary figure S7), although we note that the integration is very sensitive to curvature estimation through image processing ($\approx \pm10~\mu$N). }
\begin{figure*}
\includegraphics[width=0.95\textwidth]{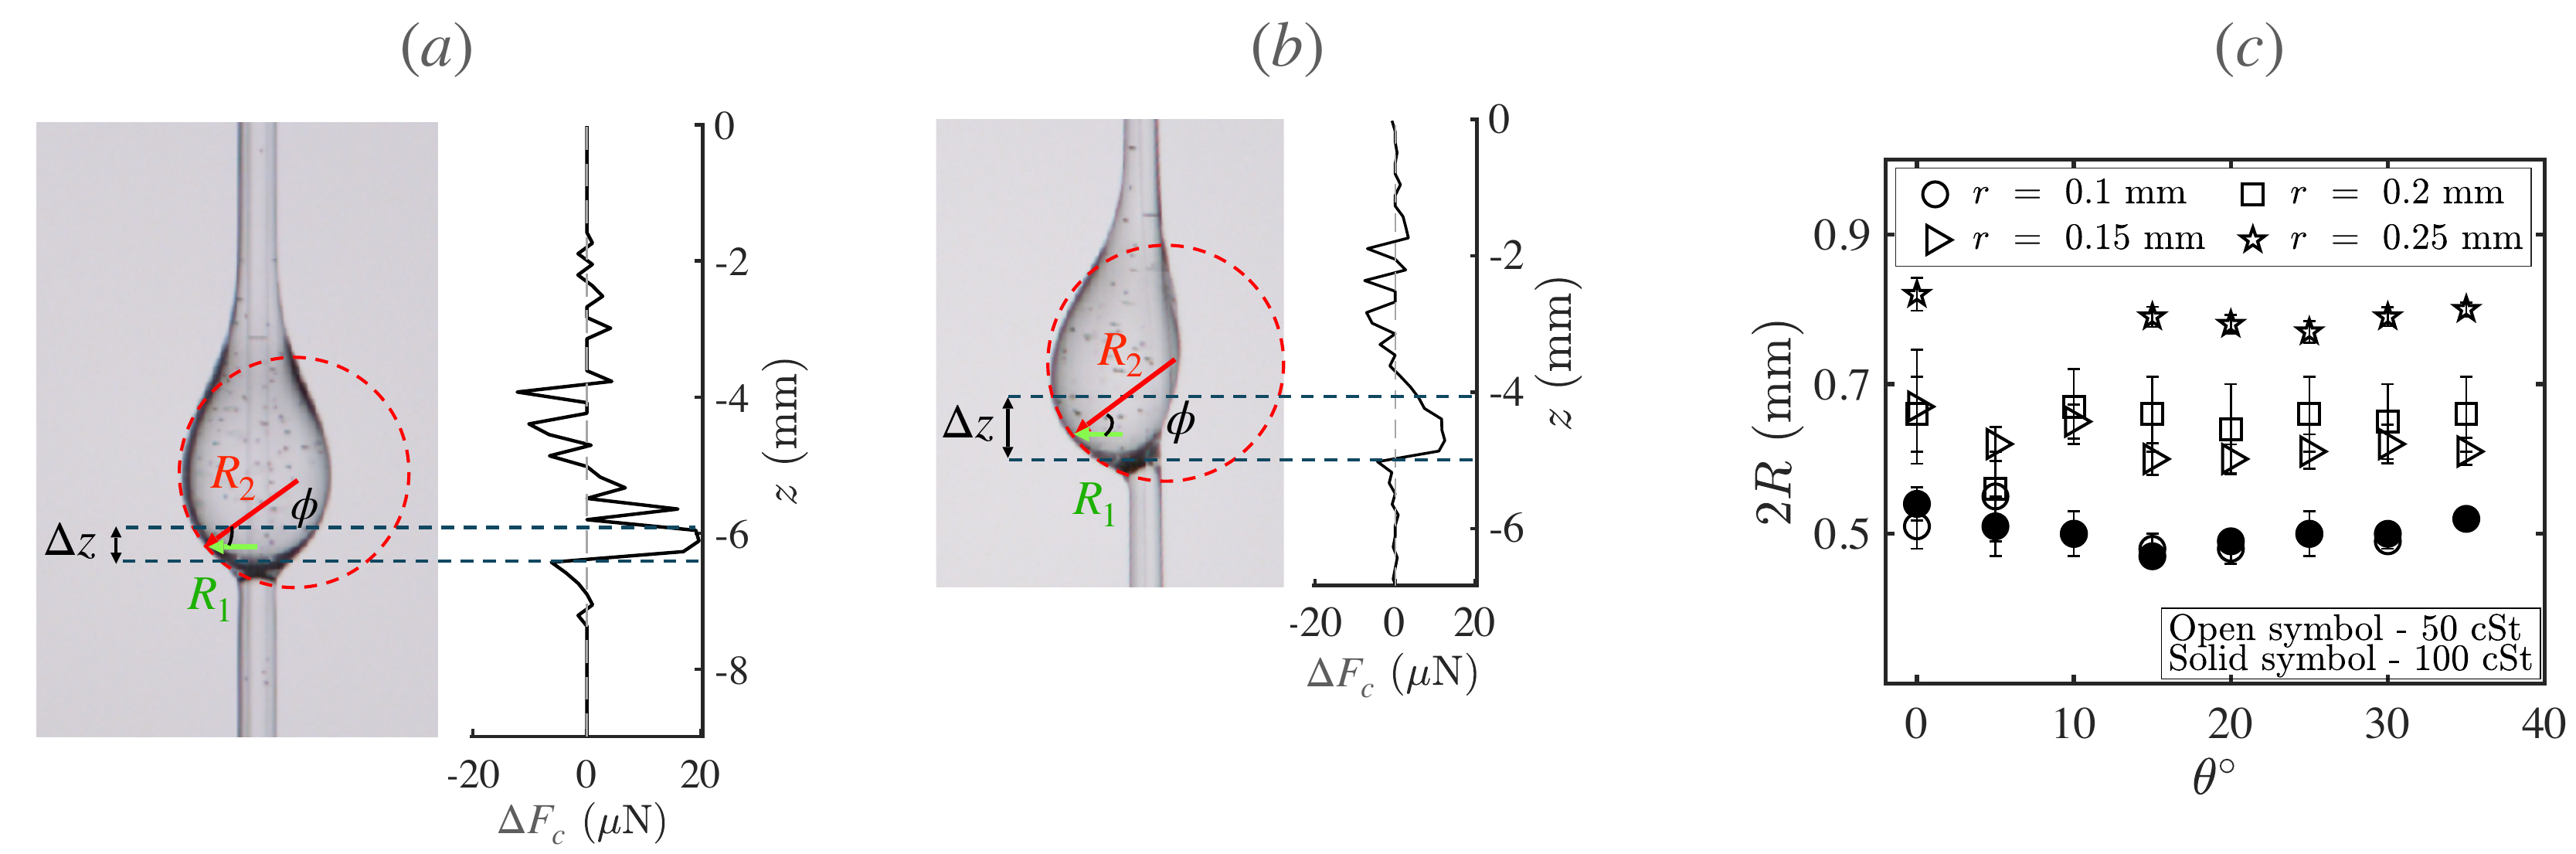}
\caption{\label{fig6_curvature} {\textbf{Curvature-induced force for Rayleigh-Plateau Instability on a wire.} (a) Experiment image of a bead and $z$ dependent upward force for $r$ = 0.1~mm, $e_n=0$ and 50~cSt silicone oil at (a) $\theta=0^\circ$, and (b) $\theta=10^\circ$
 (d) variation of the slender
cylinder diameter (2$R$) is shown as a function of $\theta$ for all cases within the Rayleigh-Plateau regime.}}
\end{figure*}

 {
 % We would like to estimate why the numerical value is close to $2\pi R \sigma$ and do so through an analytic approximation. 
%In Fig.~\ref{fig6_curvature}a,b an image from the experiment is shown next to $\Delta  F_c$ vs. $z$ to illustrate the effect of asymmetry of the droplet. 
If we continue our thought process into an analytic approximation, reminding ourselves that the assumption that the contour is not closed could be wrong then can proceed. We notice that the primary upward force arises over a finite thickness $\Delta z$ from the bottom of the droplet portion, which is of the order of $2R$ in the vertical configuration Fig.~S 9a and $4R$ in the inclined case Fig.~S 9b. In both scenarios, the outer radius satisfies $R_2 \gg R_1$ and $\phi \sim 30^\circ$.}
% \begin{equation}
% F_{c}= \int_{A}p \hat n \cdot \hat z dA = \int_{z=0}^{\lambda}\sigma \left( \frac{1}{R_1(z)} + \frac{1}{R_2(z)} \right) 2\pi R_1(z)  \sin{\phi(z)} dz
% %F_c= \int_{z=0}^{\lambda}\Delta F_c= \int_{z=0}^{\lambda}\sigma \left( \frac{1}{R_1(z)} + \frac{1}{R_2(z)} \right) 2\pi R_1(z)  \sin{\phi(z)} dz
% \label{eq:Fc_general}
% \end{equation}
% where $R_1$ and $R_2$ are the principal radii of curvature at  $z$, $\hat n$ is the unit normal vector to the surface, and  $\phi$ is the angle between the surface normal and the horizontal.
% The integration confirms that the dominant contribution to the upward force also scales as order of $2\pi R \sigma$.}
%The localized $z$-dependent force profile ($F_{c}$), plotted in Fig.~\ref{fig6_curvature}a,b, shows that the primary upward force arises over a finite thickness $\Delta z$ which is of the order of $2R$ in the vertical configuration (a) and $4R$ in the inclined case (b). In both scenarios, the outer radius satisfies $R_2 \gg R_1$ and $\phi \sim 30^\circ$.
%We now aim to calculate the main contribution to the length of $\Delta z$. To this end, a circular arc is fitted within the region $\Delta z$, and the corresponding curvature-induced force is evaluated using Equation~\ref{eq:Fc_general} for both the vertical and inclined configurations.
{
For the vertical configuration, the surface area is approximately $2\pi R_1 \Delta z$. Therefore, the curvature-induced force can be approximated as
\begin{equation}
F_{c}  \approx \frac{\sigma}{R_1} (2\pi R_1) (\frac{1}{2}) 2R  = 2\pi R \sigma.
\label{eq:Fc_vertical}
\end{equation}}

{
In the inclined configuration, the right interface contributes negligibly to the upward force. Hence, the effective area can be approximated as $\pi R_1 \Delta z$ and  $\Delta z = 4R$ as previously noted. Despite this, the net curvature-induced force still approximates to
\begin{equation}
F_{c}  \approx \frac{\sigma}{R_1} (\pi R_1) (\frac{1}{2}) 4R  = 2\pi R \sigma.
\label{eq:Fc_vertical}
\end{equation}}

{Thus, the expression $2\pi R \sigma$ provides a robust first-order approximation of the net curvature-induced force driven by asymmetry.}

% \subsection{Angle effect}
% \subsection{Eccentric effect}
\newpage
\section{SM Video captions}

\noindent
\textbf{Video 1}: Bead dynamics when $\theta=0^\circ$, $Q=350$ ml/h and $e_n=0$. Compare to Figure 2f.
\\\\
\textbf{Video 2}: Bead dynamics when $\theta=5^\circ$, $Q=350$ ml/h and $e_n=0$. Compare to Figure 2g.
\\\\
\textbf{Video 3}: Bead dynamics when $\theta=10^\circ$, $Q=350$ ml/h and $e_n=0$. Compare to Figure 2h.
\\\\
\textbf{Video 4}: Bead dynamics when $\theta=15^\circ$, $Q=350$ ml/h and $e_n=0$. Compare to Figure 2i.
\\\\
\textbf{Video 5}: Bead dynamics when $\theta=20^\circ$, $Q=350$ ml/h and $e_n=0$. Compare to Figure 2j.
\\\\
\textbf{Video 6}: Bead dynamics when $\theta=25^\circ$, $Q=350$ ml/h and $e_n=0$. Compare to Figure 2k.
\\\\
\textbf{Video 7}: Bead dynamics when $\theta=0^\circ$, $Q=300$ ml/h and $e_n=0$. Compare to Figure 3f.
\\\\
\textbf{Video 8}: Bead dynamics when $\theta=0^\circ$, $Q=300$ ml/h and $e_n=0.1$. Compare to Figure 3g.
\\\\
\textbf{Video 9}: Bead dynamics when $\theta=0^\circ$, $Q=300$ ml/h and $e_n=0.23$. Compare to Figure 3h.
\\\\
\textbf{Video 10}: Bead dynamics when $\theta=0^\circ$, $Q=300$ ml/h and $e_n=0.42$. Compare to Figure 3i.
\\\\
\textbf{Video 11}: Bead dynamics when $\theta=0^\circ$, $Q=300$ ml/h and $e_n=0.81$. Compare to Figure 3j.
\\\\
\textbf{Video 12}: Bead dynamics with microparticle when $\theta=10^\circ$, $Q=325$ ml/h and $e_n=0$. Compare to Figure 5a and 5b.
%$\\\\

% \textbf{Video 13}: Microparticle dynamics within a bead when, $Q=350$ ml/h, $\theta=0^\circ$ and $15^\circ$. 

%\bibliography{aapmsamp}% Produces the bibliography via BibTeX.
\bibliographystyle{apsrev4-2}
\bibliography{prfluidbib.bib}% Produces the bibliography via BibTeX.
\end{document}
